# Supplementary material for: SGOOP-d: Estimating kinetic distances and reaction coordinate dimensionality for rare event systems from biased/unbiased simulations
Source: arXiv:2104.13560 ancillary file (2021-09-21)
Supplement: Supplementary file 1 [file supplementary.pdf]

# Supplementary Information for "SGOOP-d: Estimating kinetic distances and reaction coordinate dimensionality for rare event systems from biased/unbiased simulations"

Sun-Ting Tsai,[1] Zachary Smith,[2] and Pratyush Tiwary*[3, a)]

[1)] *Department of Physics and Institute for Physical Science and Technology, University of Maryland, College Park 20742, USA.*

[2)] *Biophysics Program and Institute for Physical Science and Technology, University of Maryland, College Park 20742, USA.*

[3)] *Department of Chemistry and Biochemistry and Institute for Physical Science and Technology, University of Maryland, College Park 20742, USA.*

(Dated: 28 April 2021)

[a)] Electronic mail: ptiwary@umd.edu

## Supplementary Note I: Simulation details

### A. Analytical potentials set-up

The potential $U(x, y)$ governing the model with three metastable states is given by

$$\begin{aligned} U(x,y) &= W(x^6 + y^6) - G(x,x_1)G(y,y_1) \\ &\quad - G(x,x_2)G(y,y_2) - G(x,x_3)G(y,y_3) \end{aligned} \tag{1}$$

where $W = 0.0001$ and $G(x, x_0) = e^{-\frac{(x-x_0)^2}{2\sigma^2}}$ denotes a Gaussian function centered at $x_0$ with width $\sigma = 0.8$. We also build 4-state model systems, each denoted by 4A, 4B, 4C, with governing interaction potentials $U_{\mathrm{A}}$, $U_{\mathrm{B}}$, $U_{\mathrm{C}}$:

$$\begin{aligned} U_i(x,y) &= W(x^4 + y^4) + G_i(x,0.0)G'(y,0.0) \\ &\quad - G_i(x,2.0)G'(y,-1.0) - G_i(x,0.5)G'(y,2.0) \\ &\quad - G_i(x,-0.5)G'(y,-2.0) - G_i(x,-2.0)G'(y,1.0) \end{aligned} \tag{2}$$

where $G_i(x, x_0) = e^{-\frac{(x-x_0)^2}{2\sigma_i^2}}$ have widths $\sigma_i = 0.8, 1.0, 1.2$ for $i = \mathrm{A}, \mathrm{B}, \mathrm{C}$ respectively, while $G'(y, y_0) = e^{-\frac{(y-y_0)^2}{2\sigma'^2}}$ have a fixed width $\sigma' = 1.2$. The configurations corresponding to the model potentials in Eq. 1 and Eq. 2 are illustrated in the main text in Fig. 2(a)-(d).

### B. Simulation set-up

The integration timestep for the Langevin dynamics simulation was 0.01 units, and the simulation was performed at $\beta = 2.5$ for 3-state and 4-state potentials, where $\beta = 1/k_B T$. The MD results for alanine dipeptide and Ace-Ala$_3$-Nme were obtained using the software GROMACS 5.0.4[1,2], patched with PLUMED 2.4[3] with $2fs$ timestep. The temperature was kept constant at 300K for alanine dipeptide and 400K for Ace-Ala$_3$-Nme using the velocity rescaling thermostat[4]. The metadynamics parameters for each system are listed in Table. III.

## Supplementary Note II: Free energy plots for Ace-Ala$_3$-Nme

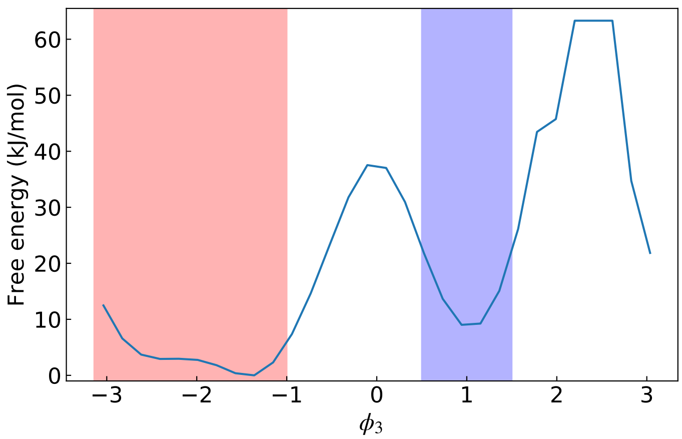


**Supplementary Figure 1** The free energy of Ace-Ala$_3$-Nme along $\phi_3$ obtained by histogramming an unbiased MD trajectory at 400K. The red and blue regions correspond to $\phi_3 \in (-3.14, -1.00]$ and $\phi_3 \in (0.5, 1.5]$. These two ranges of $\phi_3$ are integrated out to obtain free energy profiles at each metastable states.

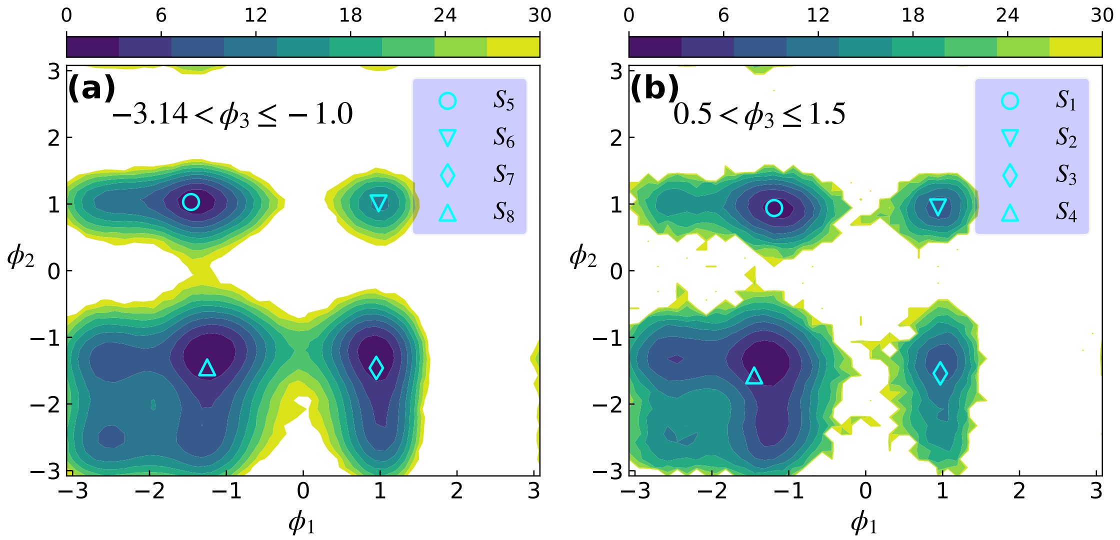


**Supplementary Figure 2** Free energy as function of $(\phi_1, \phi_2)$ obtained by making histogram of an unbiased MD trajectory where (a) $\phi_3 \in (-3.14, -1.00]$ or (b) $\phi_3 \in (0.5, 1.5]$ are selected and integrated over. The free energy profiles show four metastable states at each basin in Supplementary Figure 1.

## Supplementary Note III: Dihedral angles of metastable states for Ace-Ala$_3$-Nme used in Section III 3

| Metastable state | $\phi_1$ | $\phi_2$ | $\phi_3$ |
|---|---|---|---|
| $S_1$ | -1.19 | 0.94 | 1.08 |
| $S_2$ | 0.94 | 0.95 | 1.03 |
| $S_3$ | 0.97 | -1.54 | 1.06 |
| $S_4$ | -1.45 | -1.57 | 1.04 |
| $S_5$ | -1.46 | 1.03 | -1.72 |
| $S_6$ | 0.98 | 1.01 | -1.71 |
| $S_7$ | 0.95 | -1.46 | -1.82 |
| $S_8$ | -1.25 | -1.45 | -1.73 |

**Supplementary Table 1** The reference dihedral angles in radians for the 8 metastable states we used in SGOOP-d to estimate 28 pairs of commute distances. The first and last 4 metastable states are separated by the third dihedral angle $\phi_3$, where the first 4 have $\phi_3$ near 1 and the last 4 have $\phi_3$ near -1.7. The relative positions can be seen in the free energy plots at two different ranges of $\phi_3$.

## Supplementary Note IV: Metadynamics parameters

| Systems | $h$ | $\omega$ | $\Delta t$/MD step | $\gamma$ |
|---|---|---|---|---|
| 3-state | 0.3 ($k_BT$) | 0.2 | 200 | 3.5 |
| 4A (Fig. 2(b)) | 0.4 ($k_BT$) | 0.3 | 200 | 126 |
| 4B (Fig. 2(c)) | 0.4 ($k_BT$) | 0.3 | 200 | 6 |
| Alanine dipeptide | 1.2 (kJ/mol) | 0.2 | 500 | 5 |
| Ala3 1-d | 1.5 (kJ/mol) | 0.25 | 400 | 10 |
| Ala3 2-d | 1.5 (kJ/mol) | 0.2 | 500 | 5 |

**Supplementary Table 2** The metadynamics parameters used for simulation of Langevin dynamics with 3-state, 4-state model potentials, alanine dipeptide, and Ace-Ala$_3$-Nme (Ala3), where Ala3 1-d corresponds to biasing 1-d SGOOP-RC and Ala3 2-d corresponds to biasing 2-d SGOOP-RC. Gaussian bias kernels of starting height $h$ and width $\omega$ are added every $\Delta t$ MD steps. $\gamma$ is the bias factor for well-tempered metadynamics.

## References


[1]Herman JC Berendsen, David van der Spoel, and Rudi van Drunen. Gromacs: a message-passing parallel molecular dynamics implementation. Comp. Phys. Commun., 91(1-3): 43–56, 1995.

[2]Mark James Abraham, Teemu Murtola, Roland Schulz, Szilárd Páll, Jeremy C Smith, Berk Hess, and Erik Lindahl. Gromacs: High performance molecular simulations through multi-level parallelism from laptops to supercomputers. SoftwareX, 1:19–25, 2015.

[3]Massimiliano Bonomi, Giovanni Bussi, and Carlo Camilloni Camilloni. Promoting transparency and reproducibility in enhanced molecular simulations. Nat. Methods., 16:670–673, 2019.

[4]Giovanni Bussi, Davide Donadio, and Michele Parrinello. Canonical sampling through velocity rescaling. J. Chem. Phys., 126(1):014101, 2007.
